# Supplementary material for: Identifying Shopping Intent in Product QA for Proactive Recommendations
Source: arXiv:2404.06017 source file (2024-04-09)
Supplement: Supplementary file 1 [file appendix.tex]

\appendix
\section{Appendix}

\subsection{Approach Overview}
\begin{figure*}[ht!]
    \centering
    \includegraphics[width=0.9\textwidth]{images/spq_diag.pdf}
    \caption{\small{SPQI: For an incoming product question SPQI performs the following steps to predict whether it is an SPQ: (a) computing the question text representation using pretrained transformer models; (b) extracting the queried product (e.g. \emph{``hershey chocolate bar''}); (c) extracting its category in the product catalog (e.g. \emph{``sweets \& candy''}); (d) encoding the voice assistant response using pretrained models as in (a). In (e) -- (h) the input features are pushed through a \texttt{FFN} layer, allowing the features to be of the same dimensionality. In (i) the features are combined using the MoE approach, and are then fed into GAT's message-passing, which computes the node representation according to a computed sub-graph at batch time (j), each node representing a question. The resulting node representation in (k) is used for classifying the question as either SPQ or NSPQ using a Sigmoid layer.}}
    \label{fig:spq_approach}
\end{figure*}

\subsection{Feature List}
\begin{table}[h!]
    \centering
    \small
    \resizebox{1.0\columnwidth}{!}{
    \begin{tabular}{l p{3.5cm} p{3.5cm}}
    \toprule
    & feature & description\\
    \midrule
         1 & question text & \texttt{[CLS]} token representation from RoBERTa  \\
         2 & voice assistant answer & \texttt{[CLS]} token representation from RoBERTa  \\
         3 & product embedding & categorical feature  \\
         4 & product category embedding & categorical feature \\
         5 & parent product category embedding & categorical feature \\
         6 -- 11 & behavioral features & numerical features extracted from user's purchase history \\
    \bottomrule
    \end{tabular}    }
    \caption{List of features used in our models.}
    \label{tab:feature_list}
\end{table}

\subsection{Question Graph Construction}

\begin{figure}[ht!]
    \centering
    \includegraphics[width=0.9\columnwidth]{images/batch_subgraph.pdf}
    \caption{\small{Graph construction over a sample of questions.}}
    \label{fig:batch_graph_construction}
\end{figure}

\subsection{Multi-Stage Training}

Following GAT architecture based approaches, we combine various features that are either randomly initialized (e.g. product embeddings), or features that come from pre-trained models (e.g. textual features). In order for the models to learn appropriate representations for the randomly initialized features, we use a multi-stage training strategy as proposed in ~\cite{DBLP:conf/naacl/MengFRM21}.

\begin{itemize}[leftmargin=*]
    \item First Stage: we first freeze the parameter space for the pre-trained feature sets, and allow the model to train only the randomly initialized features for a single epoch. In the first stage we set a high learning rate $lr=0.001$ -- as the randomly initialized features do not contain any knowledge, the learning rate can be high.
    \item Second Stage: in this stage, we jointly train all of the model's parameters with a learning rate of $lr=3e-5$. We train the model until convergence, and set an early stopping criterion of a non-decreasing loss of more than 3 epochs on the validation set.
\end{itemize}

\subsection{Performance by Product Category}

Figure~\ref{fig:precision_by_category} shows the F1 score obtained by the \modelname{SPQI-Full-MoE} model for different product categories with varying number of PQs. 
We note a significant variation in terms of $F1$ score across the different product categories. The difference in performance can be an indication of how predictable are users' shopping needs on different categories. Furthermore, this shows that depending on the range of products that can be queried from a category, and possibly the frequency of purchases, the performance of our model varies. For instance, products that are typically purchased less frequently by voice, e.g. \emph{``vacuums {\&} floors''} or \emph{``parts \& accessories / refrigerator''}, have the lowest $F1$ scores. On the contrary, \emph{``dog food''} or \emph{``vitamins \& dietary''}, have significantly higher $F1$ scores.

\begin{figure*}[ht!]
     \centering
      \centering
     \subfloat{\includegraphics[width=0.48\textwidth]{images/f1_by_category_d2.pdf}\label{fig:precision_by_category}}
     \subfloat{\includegraphics[width=0.48\textwidth]{images/category_utterance_ratio.pdf}\label{fig:utterances_by_category}}
     \caption{\small{(a) F1 score of \modelname{SPQI-MoE-Full} for the different product categories. Performance varies across different categories, showing a tendency of lower performance for categories, whose product range is wider, e.g. \emph{``portable audio \& video''}. On the other hand, for product categories, e.g. \emph{``cat food''}, the model achieves high F1 scores. (b) Question distribution for the same subset of 20 product categories, which are chosen to reflect the cases where \modelname{SPQI-MoE-Full} has either high or low accuracy.}}
    \label{fig:precision_by_category}
\end{figure*}
